# Supplementary material for: DepthFocus: Controllable Depth Estimation for See-Through Scenes
Source: arXiv:2511.16993 ancillary file (2026-03-25)
Supplement: Supplementary file 1 [file supp_arxiv.pdf]

# Supplementary Materials

## DepthFocus: Controllable Depth Estimation for See-Through Scenes

Junhong Min<sup>1,†</sup>, Jimin Kim<sup>1</sup>, Cheol-Hui Min<sup>1</sup>, Minwook Kim<sup>1</sup>, Youngpil Jeon<sup>1</sup>, Minyong Choi<sup>1</sup>  
<sup>1</sup>Samsung Electronics, <sup>†</sup> Corresponding author  
junhong1.min@samsung.com

### 1. Synthetic Data Generation

We constructed a large-scale synthetic multi-layer dataset comprising approximately 500k stereo RGB pairs. This dataset includes aligned per-layer depth and disparity maps, instance and semantic masks for transmissive objects, and corresponding camera intrinsics and extrinsics.

#### 1.1. Data Generation Pipeline

Our data generation pipeline is implemented using Blender and its Python API, leveraging high-quality 3D assets sourced from BlenderKit [1]. The pipeline consists of three primary stages: (1) scene setup, (2) material and geometry variation, and (3) rendering. Figure 1 illustrates the overall workflow.

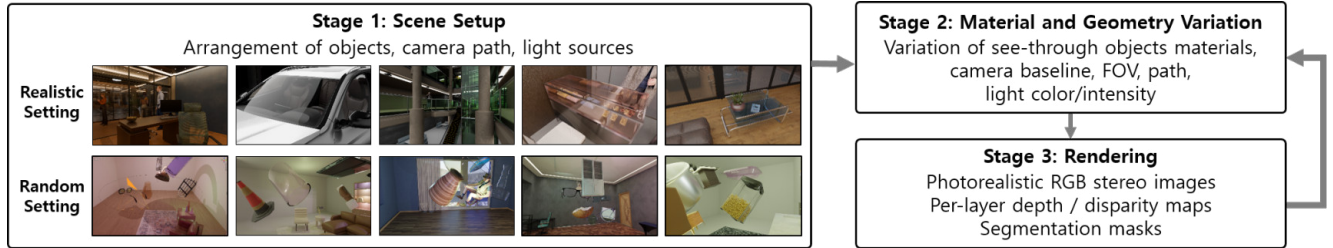

Figure 1. Synthetic data generation pipeline.

In the first stage, we prepare the base scene for rendering. To ensure diversity, we developed two distinct scene configuration protocols: a realistic setting and a randomized setting. In both settings, camera paths are procedurally generated using various primitives, including lines, circles, ellipses, and splines. In the realistic setting, objects are arranged to mimic real-world multi-layered environments. We applied manual modifications, such as object addition, removal, and repositioning, to base scenes provided by BlenderKit, while adjusting materials to fit our requirements. The scene composition includes both opaque objects and see-through entities, ranging from transparent items (e.g., windows, glass containers, acrylic tables) to porous structures (e.g., fabric-mesh chairs). Additionally, to introduce inter-frame variation, rigging animation was applied to human and vehicle assets. In the randomized setting, we employ a domain randomization strategy where canonically scaled objects are procedurally instantiated in arbitrary 3D poses within free space. This setup facilitates data acquisition from unconventional viewing angles and scale ratios rarely observed in realistic layouts, thereby enhancing the model’s robustness.

Stage 2, the material and camera variation stage, perturbs object materials and camera properties to expand dataset diversity efficiently. As shown in Figure 1, the pipeline iterates through Stages 2 and 3 for each base scene created in Stage 1. The randomized parameters and their typical ranges are:

- Camera properties: Path scale and angle, inter-frame displacement (0.01–0.3m), baseline (0.02–0.25m), and Field of View (FOV) (40–100°).
- Light properties: Color temperature, direction, and intensity.
- See-through material properties: Base color, Index of Refraction (IoR) (1.0–1.5), metallic (0.05–0.2), and roughness (0.0–0.01).

In the final stage, the pipeline renders stereo RGB images, segmentation masks, and per-layer depth maps as the camera traverses the predefined path. Since standard render passes do not natively support per-layer depth maps, we implemented a multi-pass ray-depth peeling technique utilizing Blender’s Light Path information. This method leverages the ray transmission counter (Transparent Depth) to selectively render surfaces based on their layer order. By iteratively adjusting a transparency threshold, we sequentially peel away foreground transparent layers to capture the depth of subsequent layers. For instance, a threshold of 0 captures the nearest surface, whether opaque or transparent, while a threshold of 2 penetrates the first transparent layer to capture the geometry behind it (accounting for both entry and exit surfaces). This approach allows us to systematically obtain comprehensive multi-layer depth information.

## 1.2. Dataset Diversity

Our dataset spans both indoor and outdoor environments to ensure broad coverage of real-world scenarios. Indoor scenes include bedrooms, bathrooms, living rooms, kitchens, cafes, shops, offices, warehouses, and sports areas, while outdoor scenes comprise roads and building exteriors. We prepared 263 distinct base scenes in Stage 1 and generated 3,577 unique configurations in Stage 2. To ensure object diversity, the dataset incorporates an extensive collection of 3D models, comprising over 2,000 opaque objects and more than 700 see-through objects. The see-through objects exhibit a wide range of geometric properties, including flat surfaces (e.g., windows, tables) and curved surfaces (e.g., cups, bottles, lamps). For transparent materials, we carefully controlled optical properties to achieve realistic rendering. To further enhance realism, we utilized specialized glass materials beyond the default Glass BSDF, such as scratched, smudged, and frosty glass. The training set consists of approximately 500k stereo pairs at resolutions of  $1280 \times 720$  and  $2448 \times 2048$ . Each image was rendered with high sampling rates (64 to 512 samples per pixel) to minimize noise and ensure high-fidelity transmission effects

For a more detailed visual exploration of our synthetic dataset and rendering quality, we refer readers to the [accompanying supplementary video](#).

## 1.3. Test Set

The synthetic test set comprises five distinct scenes (bedroom, office, cafe, gallery, and outdoor), covering both indoor and outdoor environments. Each scene contains 85 to 140 frames, resulting in a total of 535 frames. All frames were rendered at a resolution of  $2448 \times 2048$  with 512 samples per pixel to ensure high-fidelity image quality. To facilitate a comprehensive evaluation, we strategically placed a variety of challenging objects, including windows, display cases, glassware, and mesh chairs, within these scenes. This diverse composition enables a thorough assessment of the model’s performance across varying material properties, lighting conditions, and scene complexities.

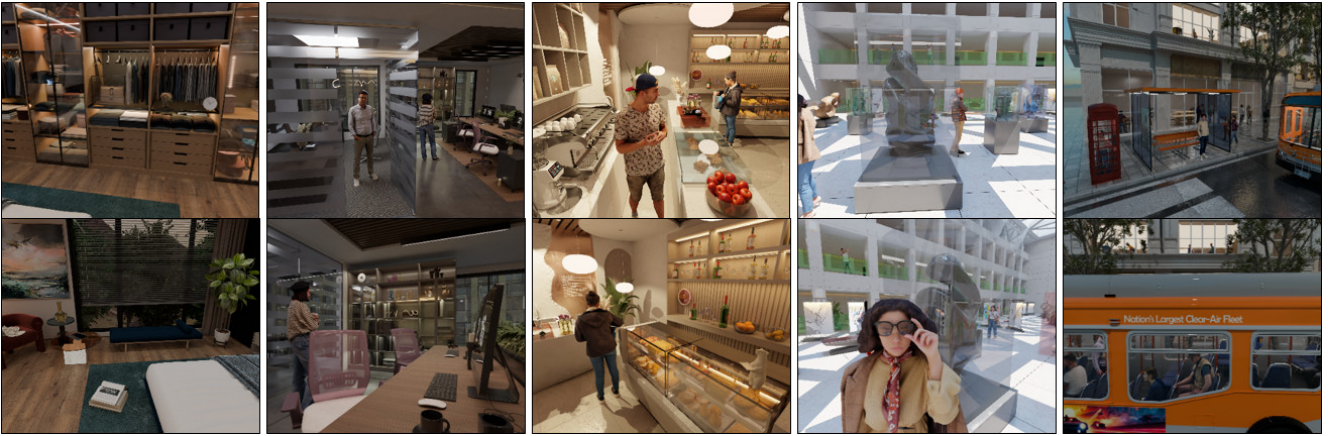

Figure 2. Configurations of our synthetic test dataset. The test set spans five diverse environments: bedroom, office, cafe, gallery, and outdoor urban areas. These scenes are designed to comprehensively cover various multi-layered real-world scenarios.

## 2. Real-World Data Generation

In this section, we detail our data acquisition system designed to generate a high-quality dataset for multi-layered depth estimation. To simulate real-world see-through scenarios in a controlled laboratory environment, we physically constructed a multi-layered scene by positioning a translucent acrylic plate in mid-air between the camera and the background objects. This setup allows us to capture precise ground truth (GT) data for both the foreground translucent surface (via geometric modeling) and the background geometry (via high-precision sensors).

### 2.1. System Configuration

To begin, Figure 3 illustrates our experimental setup for data acquisition, featuring two 6-DoF industrial robot manipulators. This dual-robot configuration is specifically designed to capture the scene from diverse viewpoints while precisely positioning a translucent object within the environment.

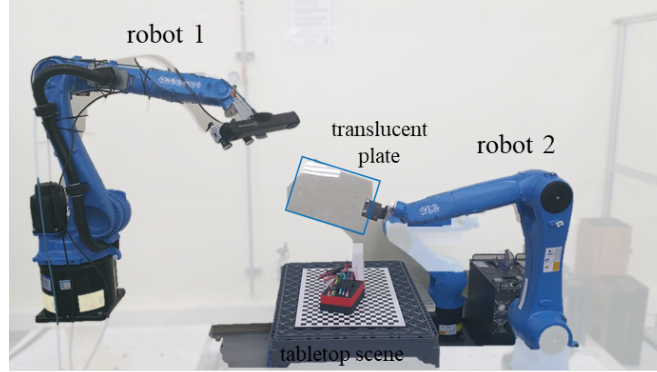

Figure 3. Real-world data acquisition setup

Specifically, for *robot1* in Figure 3, we attach a multi-camera system to its end-effector, as shown in Figure 4. This setup allows *robot1* to generate multiple camera views of the tabletop scene. The poses of *robot1* are carefully designed to optimize point cloud measurements from the Photoneo PhoXi 3D Scanner M<sup>1</sup>, considering its depth measurement range.

While *robot1* controls the 6D poses of the cameras, *robot2* is equipped with a translucent plate on its end-effector and adjusts the plate’s 6D pose to capture various translucent object measurements. As discussed in Figure 6 of the main paper, we employ two distinct levels of plate transmittance for these measurements.

### 2.2. Camera Configuration

As shown in Figure 4, our camera system attached to the end-effector of *robot1* (Figure 3) consists of two primary components: (1) a Photoneo PhoXi 3D Scanner M and (2) a stereo RGB camera system comprising two Baumer 5MP industrial RGB sensors<sup>2</sup> equipped with 4.5mm fixed focal length lenses<sup>3</sup>. The PhoXi scanner serves to provide accurate depth measurements for non-transparent objects, while the stereo camera system is employed to acquire the synchronized stereo imagery required for the dataset.

To ensure pixel-level correspondence between the depth sensor and the RGB images, we perform precise spatial alignment. We calculate the sensor-to-sensor transformation  $T_{PL} \in SE(3)$  from the Photoneo frame  $\{P\}$  to the left stereo camera frame  $\{L\}$  following the calibration procedure described in [8]. Additionally, for disparity computation, we calibrate the stereo system between  $\{L\}$  and  $\{R\}$  to obtain the intrinsic matrix  $K \in \mathbb{R}^{3 \times 3}$  and the baseline transformation  $T_{LR} \in \mathbb{R}^{3 \times 3}$  using standard stereo rectification.

### 2.3. Sensor-to-Sensor Calibration and Background GT Alignment

The generation of our ground truth relies on a hybrid approach tailored to the material properties of the scene. In this subsection, we focus on acquiring GT for the opaque background regions (i.e., the environment beneath the transparent

<sup>1</sup><https://www.photoneo.com/ko/products/phoxi-scan-m/>

<sup>2</sup><https://www.baumer.com/kr/ko/product-overview/industrial-cameras-image-processing/industrial-cameras/cx-series/vcx-i-cameras/cameras-for-demanding-image-processing-tasks/vcxg-i/vcxg-2-57c-i/p/47343>

<sup>3</sup><https://www.edmundoptics.com/p/45mm-c-series-fixed-focal-length-lens/29328/?srsltid=AfmBOoqXd-hVcZ74rglaQRLCYinaEMdAXheoSOG5glxsxTt4s-LogjMN>

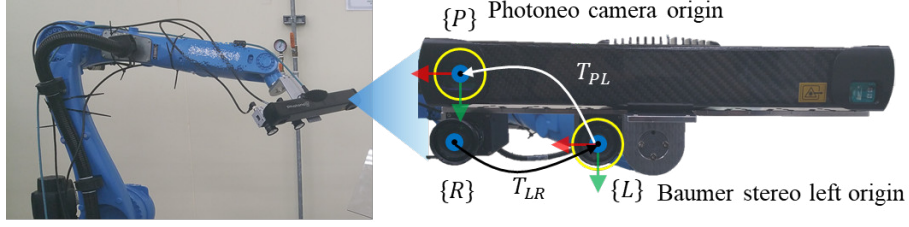

Figure 4. Multi-camera system configuration

object), where the Photoneo structured light sensor provides reliable measurements.

We align the point cloud measurement  $P_P$  from the Photoneo sensor with the left RGB image  $I_L$  using the pre-calibrated transformation  $T_{PL}$ . Subsequently, the transformed point cloud is projected onto the image plane of  $\{L\}$  using the intrinsic matrix  $K$ . This process yields a dense depth map serving as the ground truth for the non-transparent environmental geometry.

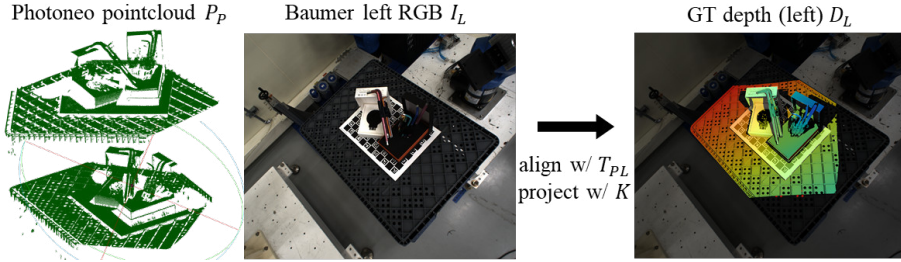

Figure 5. Pipeline for creating sensor-based ground-truth depth for opaque background regions, aligned with left stereo  $I_L$ .

## 2.4. Geometric Disparity Projection for Translucent Foreground Region

While the Photoneo sensor captures the background, it cannot reliably measure the surface depth of the transparent (translucent) plate due to the limitations of structured light on specular and transmissive surfaces. Therefore, to obtain accurate GT for the translucent foreground region, we exploit the known physical properties of the plate (i.e., a flat rectangular surface) and employ a plane fitting approach facilitated by manual annotation.

The generation process consists of four main steps designed to fuse the analytic foreground with the sensor-based background:

1. **Manual annotation:** Users manually select exactly three corresponding points on the plate corners in each stereo pair image.
2. **Triangulation:** Convert the selected 2D image points to 3D world coordinates using stereo geometry.
3. **Plane fitting:** Fit a mathematical plane to the 3D points using an SVD-based least squares method to model the plate surface.
4. **Integration:** Generate depth maps for the fitted plane and composite them over the sensor-based background measurements.

**3D point triangulation.** As shown in Figure 6a, the user first manually selects three corresponding points in both the left and right images:  $p_l^i = (u_l^i, v_l^i)$  and  $p_r^i = (u_r^i, v_r^i)$  for  $i = 1, 2, 3$ . We then perform triangulation on these three point pairs. The objective is to find the 3D point  $\mathbf{X} = [X, Y, Z, 1]^T$  that projects to each corresponding image plane point pair, represented in homogeneous coordinates as  $\langle \mathbf{p}_l^i, \mathbf{p}_r^i \rangle$ .

Given the projection matrices  $P_l = K[I|0]$  and  $P_r = K[R_{LR}|t_{LR}]$ , the triangulation is formulated as solving the linear system:

$$\mathbf{p}_l^i \times (P_l \mathbf{X}) = 0, \quad \mathbf{p}_r^i \times (P_r \mathbf{X}) = 0. \quad (1)$$

Expanding Eq. 1 yields a system  $A\mathbf{X} = 0$ , where  $A$  is a  $4 \times 4$  matrix. To solve this, we employ Singular Value Decomposition (SVD). Since user-specified points may contain minor inaccuracies, we seek the best approximation by minimizing  $\|A\mathbf{X}\|_2$  subject to  $\|\mathbf{X}\|_2 = 1$ . The solution corresponds to the last column vector of  $V$  (from  $A = U\Sigma V^T$ ).

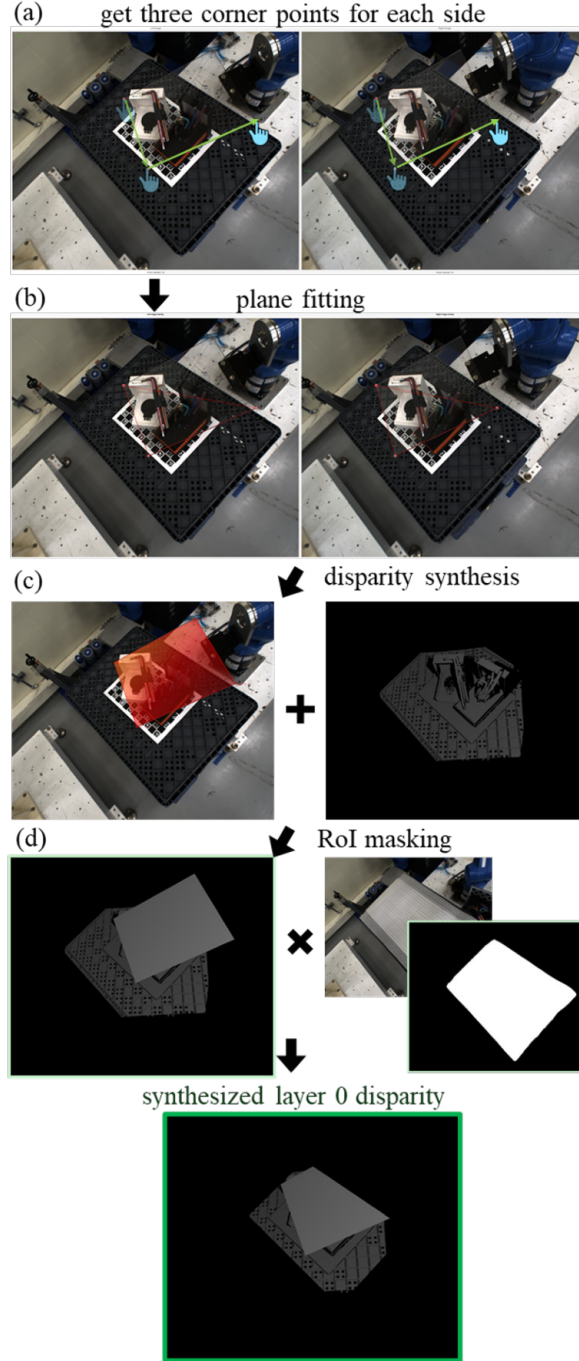

Figure 6. **Geometric disparity map generation and integration.** (a–c) Since sensors fail on transparency, the ground truth for the translucent plate is analytically derived via manual annotation of corner points and plane fitting. (d) This geometric disparity map (foreground) is then integrated with the sensor-based disparity map (background) to form the final multi-layered ground truth.

**Plane fitting.** Given three triangulated 3D points, we fit an infinite plane as shown in Figure 6b. The plane’s normal vector  $\mathbf{n}$  is computed via the cross product of the edge vectors derived from the points. The offset  $\mathbf{d}$  is then computed by evaluating the dot product  $\mathbf{d} = -\mathbf{n} \cdot \mathbf{X}_i$ .

**Generating geometric disparity map.** Using vector geometry (parallelogram law), we compute the fourth 3D corner point  $\mathbf{X}_4$  and reproject all four corners onto the left camera image plane. Using a ray-casting algorithm, we identify pixels

within this projected quadrilateral. This process generates geometric depth and disparity maps specifically for the translucent plate region, as demonstrated in Figure 6c.

**Final depth map integration.** Finally, we integrate the analytically derived plate disparity with the sensor-based background disparity maps generated in Sec. 2.3. The geometric disparity map (foreground) is overlaid onto the Photoneo-based GT map (background). Since the Photoneo camera’s measurement range extends only up to the tabletop, we apply a region-of-interest (RoI) mask to the integrated depth map to produce the final clean ground truth, as illustrated in Figure 6d.

## 2.5. Real-World Data Samples

We perform the aforementioned data acquisition procedure across five distinct scenes: {Wrenches, Plants, Car, Toys 1, Toys 2}, as illustrated in Figure 7. As detailed in the main paper, we employ two distinct levels of plate transmittance to vary the difficulty. Notably, the high-transmittance case (approx. 80%) poses a significant challenge; as shown in Figure 8, the plate becomes nearly invisible in standard RGB imagery, making it extremely difficult to detect based on visual cues alone. For real-world evaluation, we provide two layers of ground truth disparity corresponding to these transmissivity levels, enabling a rigorous assessment of performance under varying optical visibility.

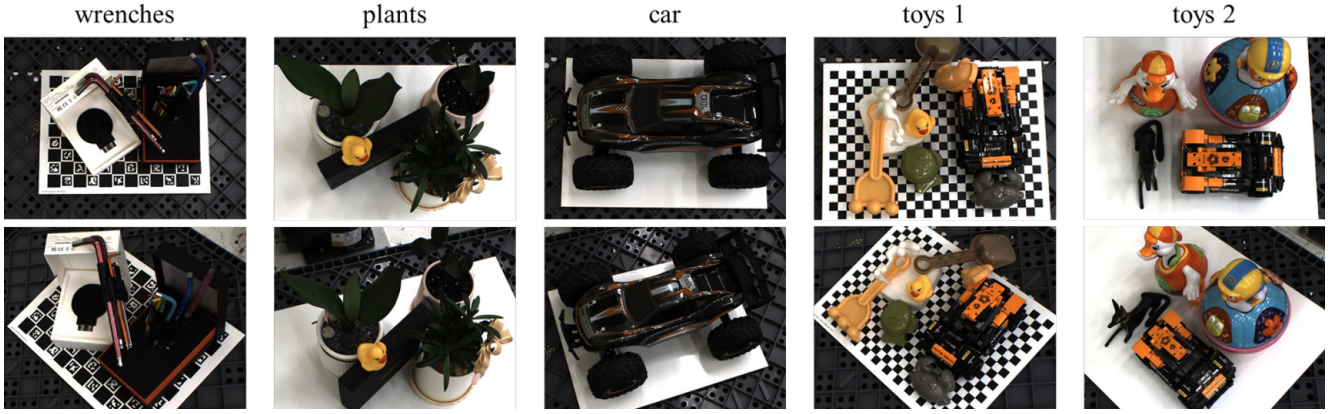

Figure 7. Real-world dataset samples

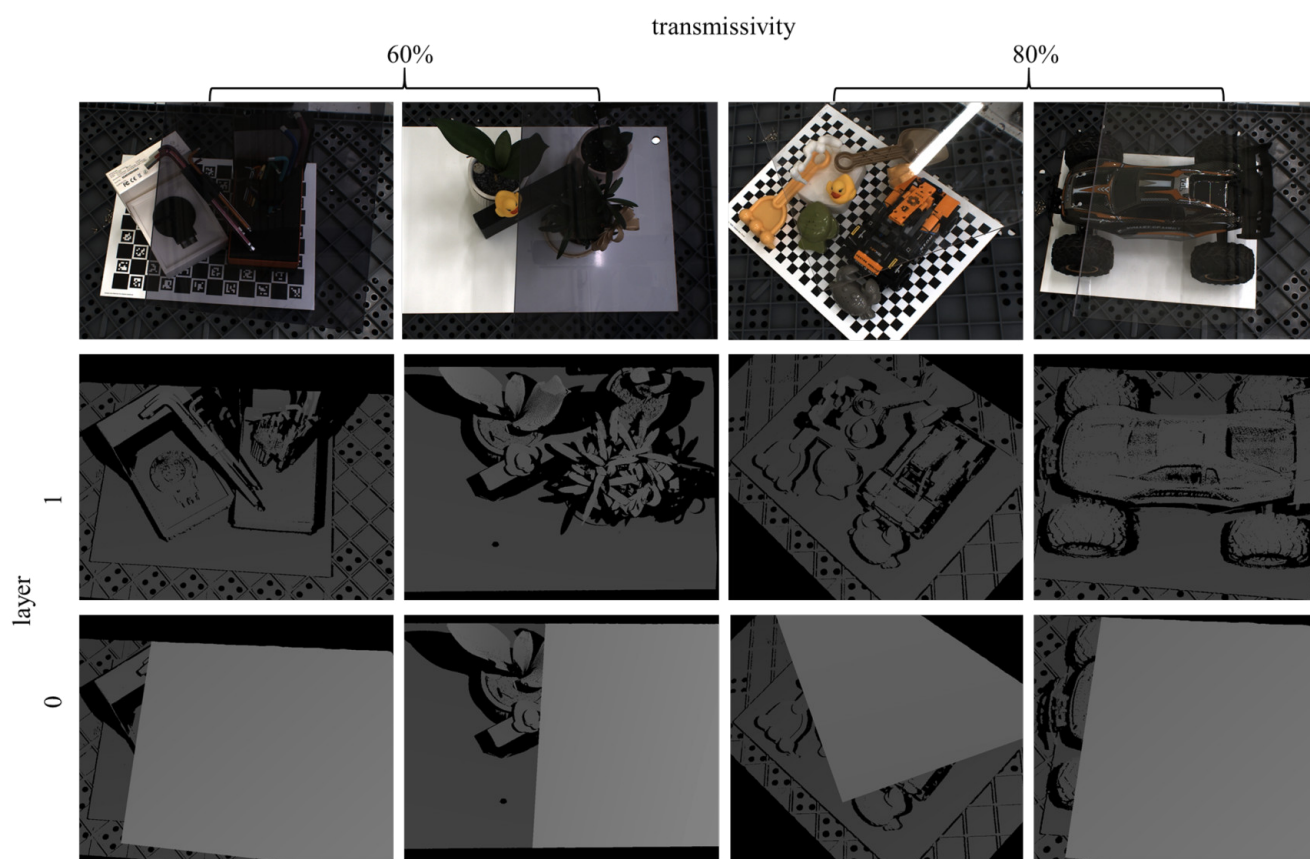

Figure 8. Transmissivity of translucent plates and corresponding GT disparity labels

### 3. Loss Function Details

Our total loss extends the baseline S<sup>2</sup>M<sup>2</sup> [9] formulation by introducing a weighted disparity loss, an auxiliary segmentation loss, and a Mixture-of-Experts (MoE) balancing loss. The final objective  $\mathcal{L}_{\text{total}}$  is a weighted sum of these components:

$$\mathcal{L}_{\text{total}} = \lambda_D \mathcal{L}_D + \lambda_O \mathcal{L}_O + \lambda_C \mathcal{L}_C + \lambda_{\text{PMC}} \mathcal{L}_{\text{PMC}} + \lambda_{\text{Seg}} \mathcal{L}_{\text{Seg}} + \lambda_{\text{Bal}} \mathcal{L}_{\text{Bal}}. \quad (2)$$

For the components shared with the baseline, we follow the original formulations for occlusion loss ( $\mathcal{L}_O$ ), confidence loss ( $\mathcal{L}_C$ ), and PMC loss ( $\mathcal{L}_{\text{PMC}}$ ) [9], as their roles remain unchanged. We provide details on our proposed weighted disparity loss  $\mathcal{L}_D$  and the new auxiliary losses ( $\mathcal{L}_{\text{Seg}}$ ,  $\mathcal{L}_{\text{Bal}}$ ) below. We empirically set the weights as follows:

$$\lambda_D = 1, \quad \lambda_{\text{PMC}} = 1, \quad \lambda_C = 0.1, \quad \lambda_O = 0.1, \quad \lambda_{\text{Seg}} = 0.5, \quad \lambda_{\text{Bal}} = 10^{-2}.$$

This weighting strategy emphasizes disparity estimation and PMC consistency as primary objectives, while auxiliary terms provide regularization and training stability.

#### 3.1. Weighted Disparity Loss

We employ a weighted L1 loss to supervise the disparity estimation. While standard disparity loss treats all pixels equally, we introduce a regional weighting mask to emphasize critical regions such as edges and transmissive areas, which are particularly challenging in see-through scenes. The total disparity loss  $\mathcal{L}_D$  is computed as the sum over the initial estimate and  $T$  refinement stages:

$$\mathcal{L}_D = \mathcal{L}_D^{\text{init}} + \sum_{t=1}^T \mathcal{L}_D^{(t)}. \quad (3)$$

For each stage, the loss is defined as the weighted L1 distance between the predicted disparity  $D^{(t)}$  and the ground truth  $D^{\text{gt}}$ :

$$\mathcal{L}_D^{(t)} = \frac{1}{|H \times W|} \sum_{(i,j)} M_{ij} \cdot |D_{ij}^{(t)} - D_{ij}^{\text{gt}}|. \quad (4)$$

Here,  $M_{ij}$  denotes the pixel-wise weighting mask designed to focus the model on structurally important and ambiguous areas. It is formulated as:

$$M_{ij} = (1 + 0.5w_{\text{edge}}) \cdot (1 + 0.5w_{\text{nonocc}}) \cdot (1 + 0.5w_{\text{trans}}), \quad (5)$$

where the weights are defined as follows:

- $w_{\text{edge}} = 1$  for pixels on disparity edges (identified where gradient magnitude  $\geq 5$  via a Sobel filter).
- $w_{\text{nonocc}} = 1$  for non-occluded pixels.
- $w_{\text{trans}} = 1$  for pixels located within transmissive regions.

This masking strategy ensures that the model prioritizes fine geometric details and correctly resolves depth in transparent regions, rather than being dominated by large homogeneous areas.

#### 3.2. Auxiliary Segmentation Loss

To explicitly guide the network in distinguishing between different material properties, we introduce an auxiliary segmentation loss,  $\mathcal{L}_{\text{Seg}}$ . This loss supervises distinct segmentation heads to identify reflection and transmissive regions compared to the opaque background. We employ a combination of Binary Cross-Entropy (BCE) and Dice losses to handle class imbalance effectively. The loss is defined as:

$$\mathcal{L}_{\text{Seg}} = \mathcal{L}_{\text{BCE}}(S_{\text{pred}}, S_{\text{gt}}) + \mathcal{L}_{\text{Dice}}(S_{\text{pred}}, S_{\text{gt}}), \quad (6)$$

where  $S_{\text{pred}}$  and  $S_{\text{gt}}$  represent the predicted and ground truth segmentation maps, respectively. This supervision enables the network to learn the distinct visual characteristics of see-through materials, thereby reducing ambiguity in depth estimation.

### 3.3. MoE Load Balancing Loss

Our architecture incorporates a Mixture-of-Experts (MoE) layer to conditionally route features. To ensure efficient utilization of all experts and prevent the "collapse" problem where the router favors only a few specific experts, we incorporate a load balancing loss  $\mathcal{L}_{\text{Bal}}$ .

Our router network produces soft routing weights  $\{w_k\}_{k=1}^K$  for each input token. We aim to balance the expert usage across the entire batch, rather than for individual tokens. Let  $\bar{P}_k$  be the average routing probability assigned to expert  $k$  across a batch of  $B$  tokens:  $\bar{P}_k = \frac{1}{B} \sum_{i=1}^B w_k^{(i)}$ . To encourage a uniform distribution of expert usage, we minimize the squared difference between the average probability and the uniform target  $\frac{1}{K}$ :

$$\mathcal{L}_{\text{Bal}} = \alpha \sum_{k=1}^K \left( \bar{P}_k - \frac{1}{K} \right)^2, \quad (7)$$

where  $K$  is the number of experts and  $\alpha$  is a scaling hyperparameter. Minimizing this objective discourages the router from dropping specific experts, promoting balanced load distribution across the batch while allowing specialized routing for individual tokens.

## 4. Implementation Details

### 4.1. Training Strategy

We train our model on a combined dataset consisting of 2M public single-disparity stereo pairs and our 0.5M synthetic multi-layered stereo pairs. The public datasets include SceneFlow [7], TartanAir [16], CREStereo [4], FoundationStereo [17], IRS [15], Falling Things [14], Virtual KITTI 2 [2], DrivingStereo [19], SMD-Net [13], and other real-world datasets [8, 10, 11, 12]. Since the synthetic dataset provides complete multi-layer annotations essential for conditional disparity learning, it is oversampled by a factor of 10 relative to the public data. This strategy ensures that the primary training signal is derived from high-quality multi-layer supervision, while the large-scale public datasets serve as auxiliary data to enhance scene diversity and generalization.

The models are trained for 1M iterations on  $768 \times 512$  patches with a total batch size of 8 on H100 GPUs. Upon convergence, we perform a multi-resolution fine-tuning stage for an additional 100k iterations using the same dataset composition but with larger crop sizes ( $1024 \times 768$  and  $2048 \times 1536$ ) and a batch size of 24. This two-stage approach significantly improves detail fidelity and robustness across varying scales.

### 4.2. Data Curation for Single-Disparity Datasets

A core challenge in our framework is adapting large-scale public stereo datasets (approx. 2M pairs), which provide only single-disparity annotations, for our conditional model. To address this, we map the condition parameter  $c \in [0, 1]$  linearly to a global reference disparity:

$$d_{\text{ref}}(c) = (1 - c) d_{\text{max}}.$$

Here,  $c = 0$  corresponds to the near bound ( $d_{\text{max}}$ ) and  $c = 1$  to the far bound (0). Given a scene with a disparity range  $[d_{\text{min}}^{\text{scene}}, d_{\text{max}}^{\text{scene}}]$ , we sample  $c$  near the endpoints with a margin such that  $d_{\text{ref}}$  lies outside the scene-specific range. This enables conditional learning from single-annotation datasets by treating them as limit cases:

- **Type 1: Opaque/Near-Surface.** Standard datasets typically represent the first visible surface. We treat these as the "opaque" limit. **Conditioning:** We sample  $c$  near 0 such that  $d_{\text{ref}} > d_{\text{max}}^{\text{scene}}$ , aligning the model's "nearest surface" state with the dataset's ground truth.
- **Type 2: Transparent/Background.** For datasets representing background layers (or when treating the single disparity as the farthest layer), we treat them as the "transparent" limit. **Conditioning:** We sample  $c$  near 1 such that  $d_{\text{ref}} < d_{\text{min}}^{\text{scene}}$ , aligning the model's "background" state with the dataset's ground truth.

This curated utilization of single-disparity datasets complements our 0.5M synthetic multi-layered dataset, significantly increasing the diversity and efficiency of the training corpus.

### 4.3. Condition Sampling

Our multi-layered synthetic dataset allows for explicit sampling across the entire range of  $c \in [0, 1]$  because multiple disparity layers are available. To ensure the model masters both the endpoints (first visible surface vs. background) and the intermediate transitions, we adopt a mixed sampling strategy:

- **25% Endpoint Sampling:** We set  $c = 0$  or  $c = 1$  to reinforce the nearest-surface and farthest-background estimation capabilities.
- **50% Boundary-Aware Sampling:** We sample  $c$  from distributions concentrated around the disparity values of annotated multi-layer boundaries, encouraging precise discrimination in complex transition regions.
- **25% Uniform Sampling:** We sample  $c$  uniformly from  $[0, 1]$  to ensure robust interpolation capability for arbitrary user inputs.

### 4.4. Data Augmentation

We employ targeted augmentations to improve robustness against photometric and geometric variability common in real-world stereo captures:

- **Photometric transformations:** Random blur/sharpen, gamma adjustments, and additive noise are applied to model variations in image quality, lighting conditions, and sensor noise.
- **Geometric transformations:** Small random rotations are applied to account for minor camera tilts or rectification misalignments.
- **Disparity perturbations:** We introduce controlled vertical offsets ( $[-4, +4]$  pixels) and horizontal offsets ( $[-10, +10]$  pixels) to simulate imperfect rectification, thereby improving the model's tolerance to alignment errors.

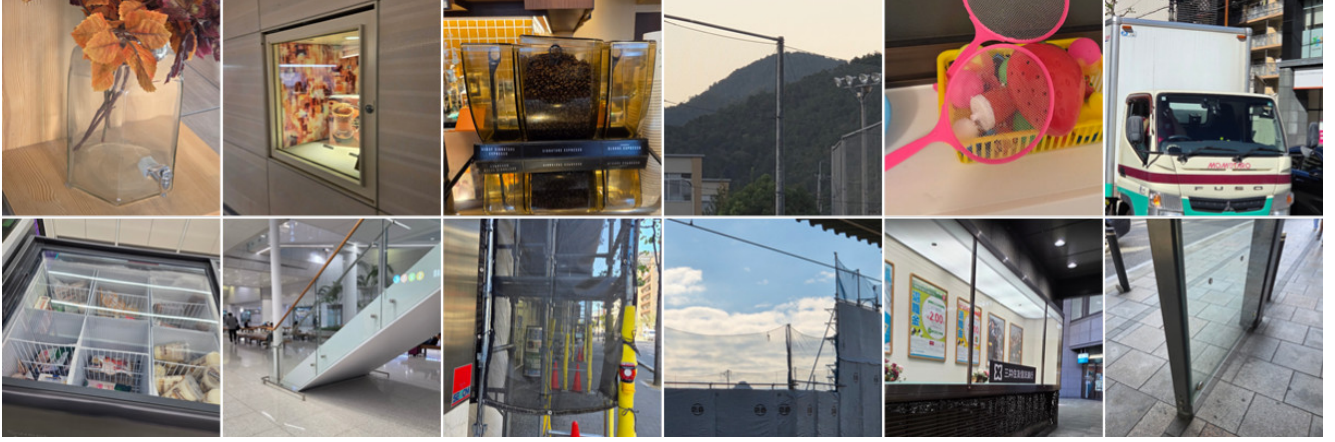

Figure 9. **Samples from our auxiliary segmentation dataset.** The dataset captures a wide variety of real-world see-through materials to supervise the segmentation branch. Examples include typical transparent objects (e.g., glass, plastic), semi-transparent porous structures (e.g., mesh, nets), and reflective surfaces.

#### 4.5. Auxiliary Segmentation Data

To supervise the auxiliary segmentation loss ( $\mathcal{L}_{\text{Seg}}$ ), we utilized a combination of existing public datasets for glass and mirror segmentation [3, 5, 6, 18] and a custom-collected dataset. Our custom dataset comprises 5,000 images captured with a standard commercial camera, explicitly curated to cover a broad spectrum of challenging see-through modalities. As illustrated in Figure 9, the dataset includes not only typical transparent objects (e.g., glass windows, plastic containers) but also complex semi-transparent structures with mesh-like textures (e.g., fabrics, insect screens) and highly reflective surfaces like mirrors. This diverse composition allows the segmentation head to learn robust features for distinguishing between refractive transmission, geometric permeability, and opaque surfaces.

## 5. Experiments

### 5.1. Auxiliary Segmentation Loss Effect on Real Datasets

This section serves as a supplementary experiment to the ablation study presented in the main paper. In our previous analysis on synthetic benchmarks, the auxiliary segmentation loss showed marginal improvements, primarily due to the limited distribution shift between training and testing sets in the synthetic domain. However, we observe that this loss plays a crucial role when generalizing to real-world scenes, specifically in aiding the network to recognize transparent surfaces.

Table 1 presents the quantitative comparison. It is important to note that a lightweight version of our model was used for this ablation to isolate the loss effect, resulting in a performance gap compared to the full model used in the main benchmark. Nevertheless, the relative impact of the segmentation loss is evident. The model trained without the segmentation loss fails almost completely in detecting transparent surfaces (see Transmissive First), exhibiting a Bad-4 error rate of over 97%. In contrast, the base model trained with the segmentation loss demonstrates improved recognition capabilities, recovering approximately 10–15% of valid pixels in these challenging transparent regions (reducing Bad-4 from 97.49 to 88.92). This confirms that explicit segmentation guidance is essential for handling material-based depth ambiguity in real-world environments.

| Ablation            | No Plate     |              | Plate (Transmittance 60%) |              |               |                |              |              |
|---------------------|--------------|--------------|---------------------------|--------------|---------------|----------------|--------------|--------------|
|                     | All          |              | Opaque                    |              | Transmissive  |                |              |              |
|                     | (c=0)        | (c=1)        | (c=0)                     | (c=1)        | First (c=0)   |                | Last (c=1)   |              |
|                     |              |              |                           |              | Bad-4         | Bad-8          | Bad-4        | Bad-8        |
| <b>Base Model</b>   | 1.73         | 2.83         | 3.78                      | 3.79         | 88.92         | 85.57          | 7.29         | 5.06         |
| <b>(-) Seg Loss</b> | 1.81 (+0.08) | 1.79 (-0.02) | 3.04 (-0.74)              | 2.28 (-0.55) | 97.49 (+8.57) | 96.42 (+10.85) | 7.98 (+0.69) | 5.53 (+0.47) |

Table 1. **Ablation study on our real benchmark.** We evaluate the impact of the auxiliary segmentation loss using a lightweight model. While the loss has minimal effect on opaque regions, it significantly improves the detection of transparent surfaces (Transmissive First), reducing the error rate by roughly 11% compared to the model without the loss. Values in parentheses indicate the performance degradation (positive value) or improvement (negative value) relative to the Base Model.

### 5.2. Sensitivity Analysis of Depth Transition Profiles w.r.t. User Intent Parameter $c$

In this section, we analyze the continuous behavior of depth estimation as the user intent parameter  $c$  varies. To visualize the depth evolution, we select three representative points located in multi-layered regions (marked in Red, Blue, and Green in Figure 10) and plot their estimated stereo disparity and confidence scores while sweeping  $c$ .

As illustrated in Figure 10, the disparity profiles (bottom row) reveal that the depth values do not switch discretely in a binary manner; instead, they exhibit a step-like transition behavior. The transition occurs rapidly over a relatively short interval of  $c$ , while the estimated depth remains constant and stable outside this transition window. This indicates that our model maintains consistent depth estimation for a given focus layer until the user intent shifts significantly. For a more comprehensive visualization of this continuous depth evolution, we refer readers to the [accompanying supplementary video](#).

Crucially, we observe a strong correlation between the transition regions and the model’s uncertainty. The confidence plots demonstrate that the estimated confidence drops significantly only within these narrow transition intervals where the depth values are intermediate and potentially inaccurate. This characteristic allows for effective outlier rejection; as shown in the third row of Figure 10, invalid depth estimates produced during layer switching can be cleanly filtered out based on confidence scores, preserving high-quality reconstruction for the selected focus distance.

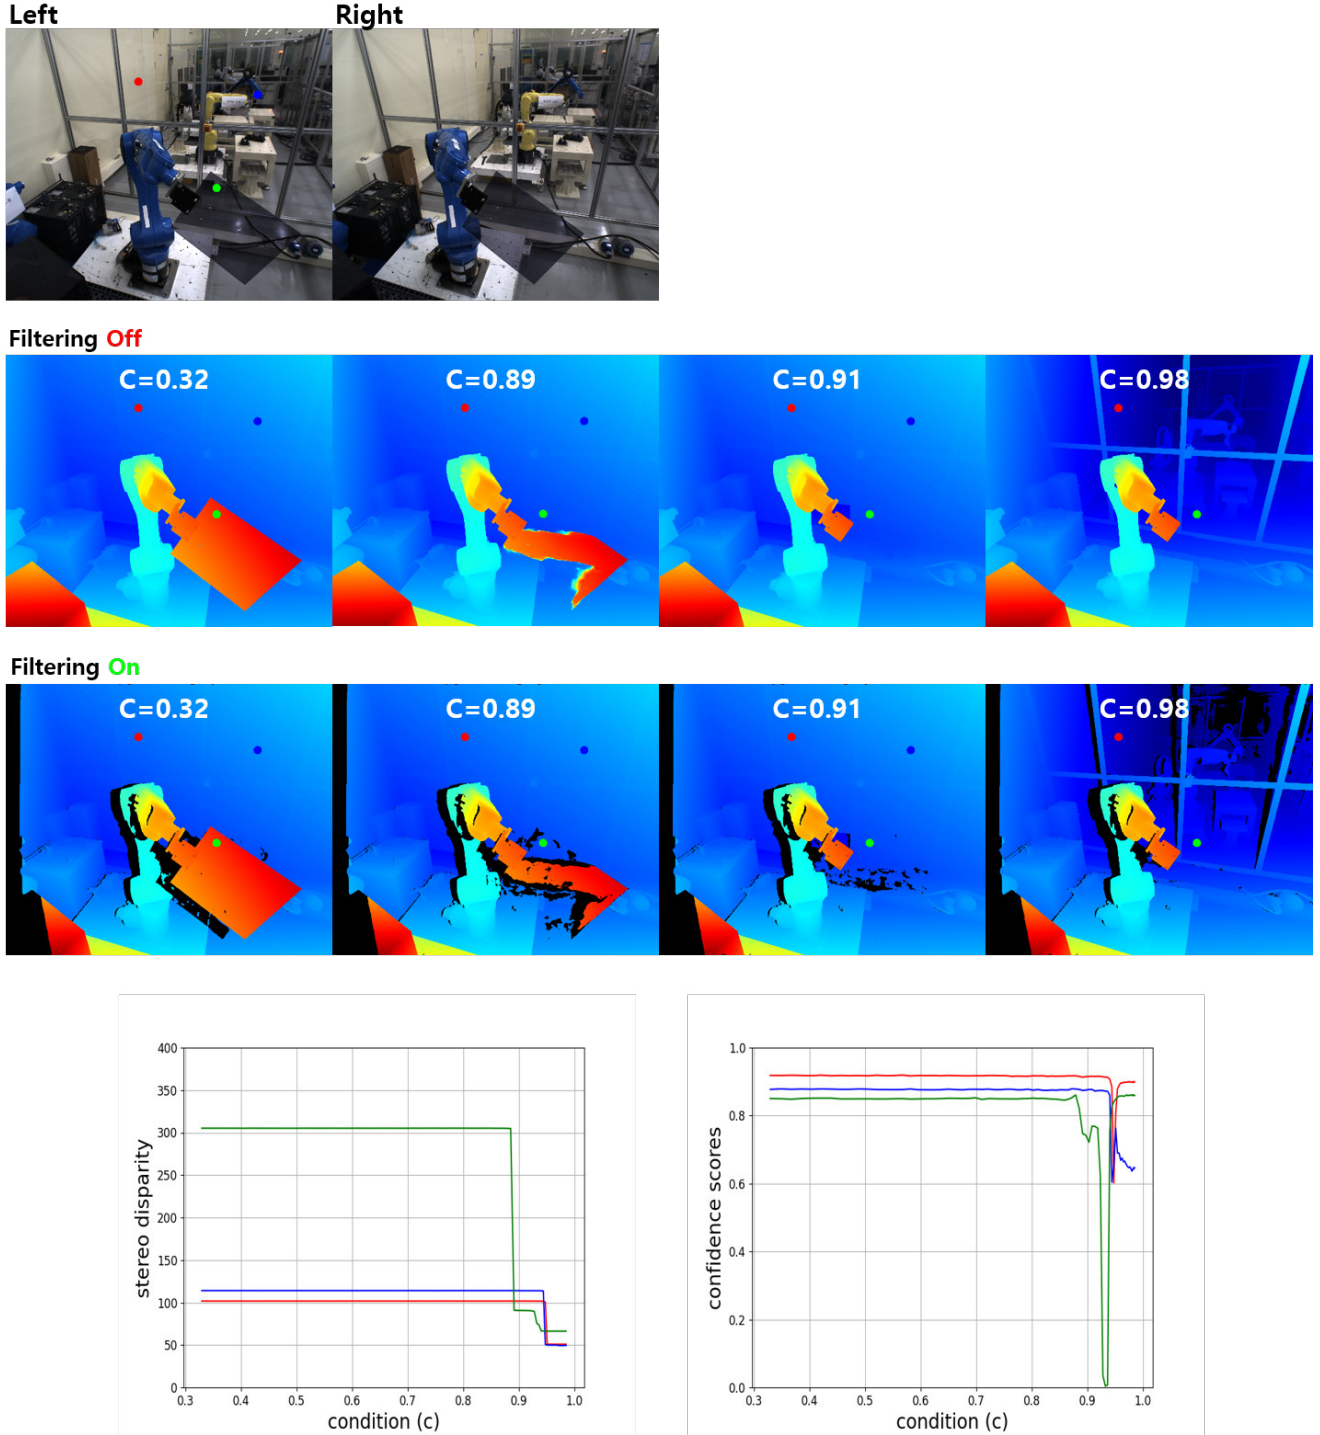

Figure 10. **Sensitivity analysis of depth transition profiles.** (Top row) Input stereo images. (Second row) Estimated depth maps corresponding to four different values of the user intent parameter  $c$ . (Third row) Filtered depth maps where pixels with low confidence scores are removed. (Bottom) Disparity and confidence profiles for three specific points (marked in Red, Blue, and Green) within the multi-layered region. The plots show a step-like disparity transition as  $c$  varies. Notably, the confidence score drops significantly during the transition interval, while remaining high in stable regions, demonstrating that inaccurate intermediate values can be effectively filtered.

### 5.3. Generalization to Real-World Scenes and Failure Analysis

We evaluate DepthFocus on our in-house dataset captured in diverse indoor environments to validate its generalization capability beyond synthetic training data. Figures 11 to 13 illustrate successful depth adaptation in multi-layered scenes. Our model effectively adjusts the estimated depth according to the user intent parameter  $c$ , demonstrating robust performance not only on typical transparent materials like plastic bowls and glass cups but also on fine geometric structures such as the mesh fabric of an office chair (Figure 11) and window insect screens (Figure 13). Furthermore, the model maintains stability even in high-contrast scenarios, such as indoor views looking outdoors where regions exhibit strong saturation.

Figure 14 highlights the robustness of our method on mirrors and highly reflective surfaces. In these scenarios, the model consistently maintains the depth of the physical reflective surface regardless of variations in the user intent parameter, correctly avoiding the estimation of virtual depth from reflected objects.

Despite these successes, we analyze representative limitations in Figure 15. Observed failures include missed detections on textureless transparent objects and floating artifacts where reflection and transmission layers are indistinguishable. Second, we observe view-dependent inconsistencies. Notably, this limitation affects even objects that are successfully detected in our success cases; a transparent surface that is correctly recognized from one viewpoint may fail to be detected when viewed from a different angle. This highlights the sensitivity of single-view cues to changes in lighting and reflection angles.

We attribute these limitations to two primary factors beyond simple model incapacity. First, there exists a sim-to-real gap; synthetic datasets often simplify the complex optical interplay of transmission and reflection. Consequently, the model has not fully learned the intricate statistical characteristics of real-world see-through regions, suggesting a need for training on more diverse real-world data.

Second, and more fundamentally, the task entails inherent ambiguity that challenges even biological vision. Humans often struggle to resolve overlapping transparent layers from a single static viewpoint. To resolve such ambiguity, humans typically rely on active perception—utilizing motion parallax by moving their heads or seeking tactile feedback to verify surface existence. In this context, the observed failure cases highlight the intrinsic difficulty of single-view estimation. This suggests that addressing these edge cases requires a comprehensive approach that goes beyond static image cues, potentially incorporating temporal information or interactive perception to achieve human-level reliability.

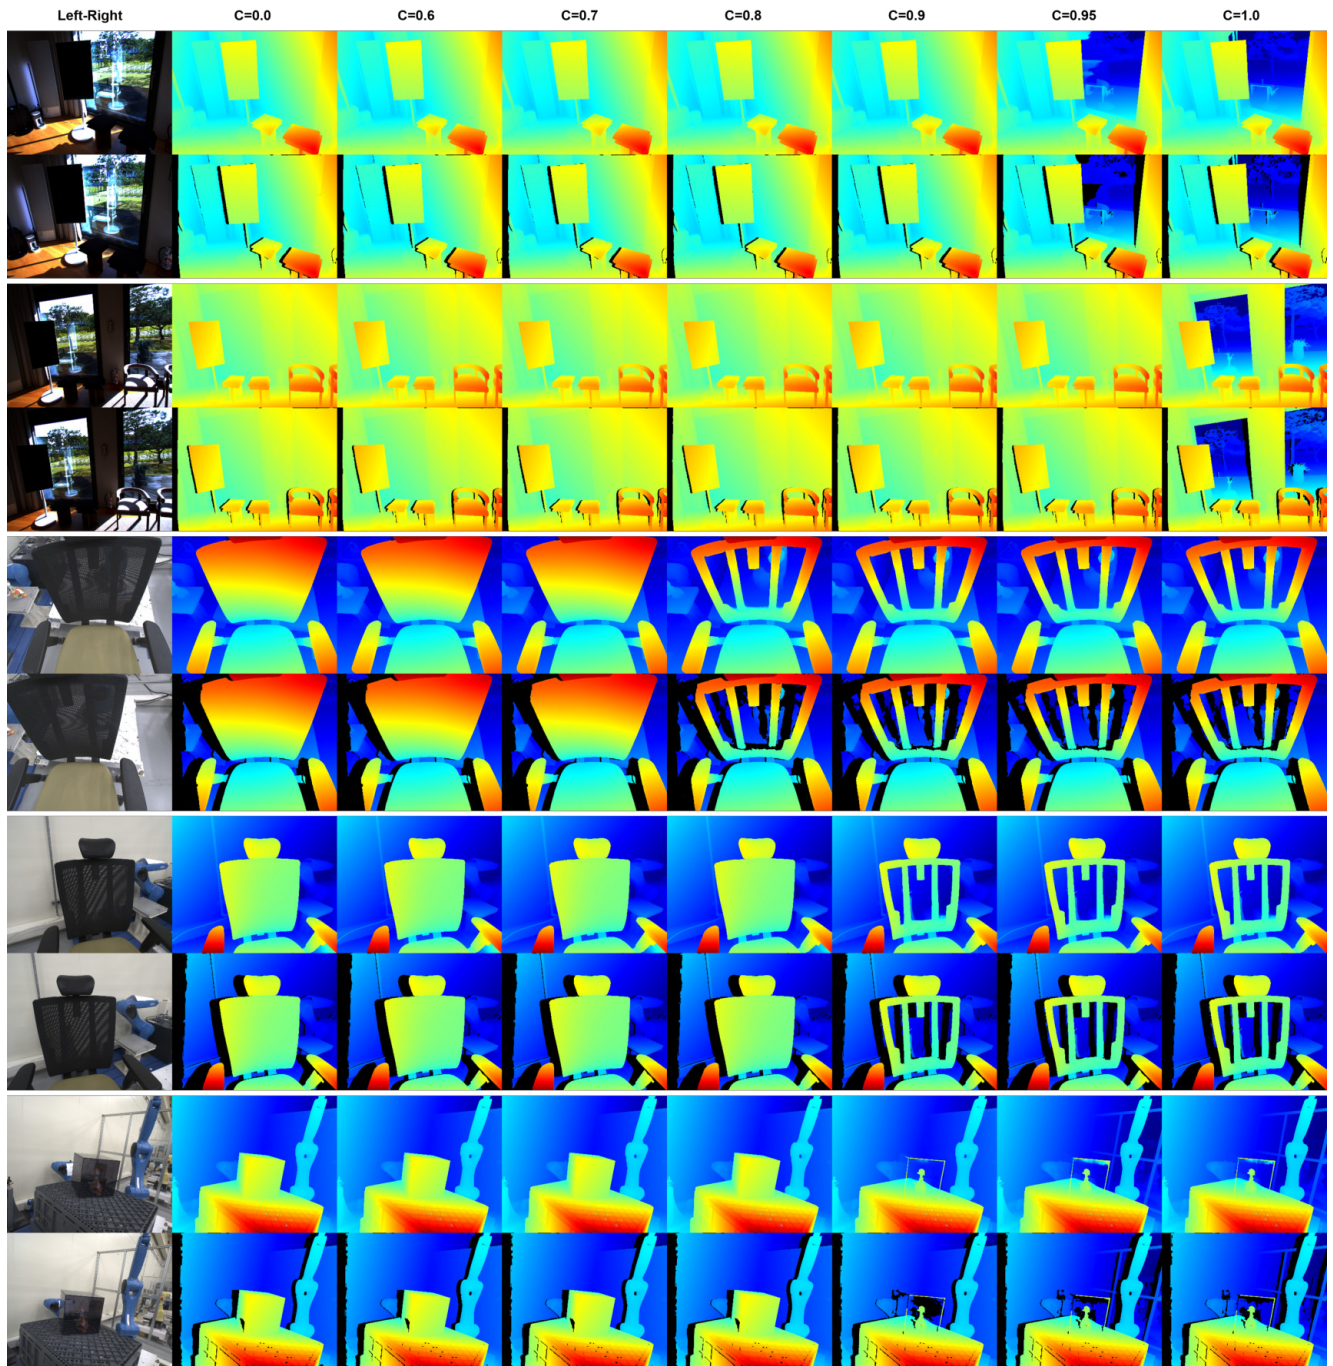

Figure 11. **Generalization to real-world scenes (1)**. Qualitative results on diverse indoor environments. **DepthFocus** effectively handles not only typical transparent objects like plastic and glass but also fine geometric structures, such as the mesh fabric of an office chair. The estimated depth maps adapt dynamically to the user intent parameter  $c$ , successfully resolving the depth of semi-transparent textures.

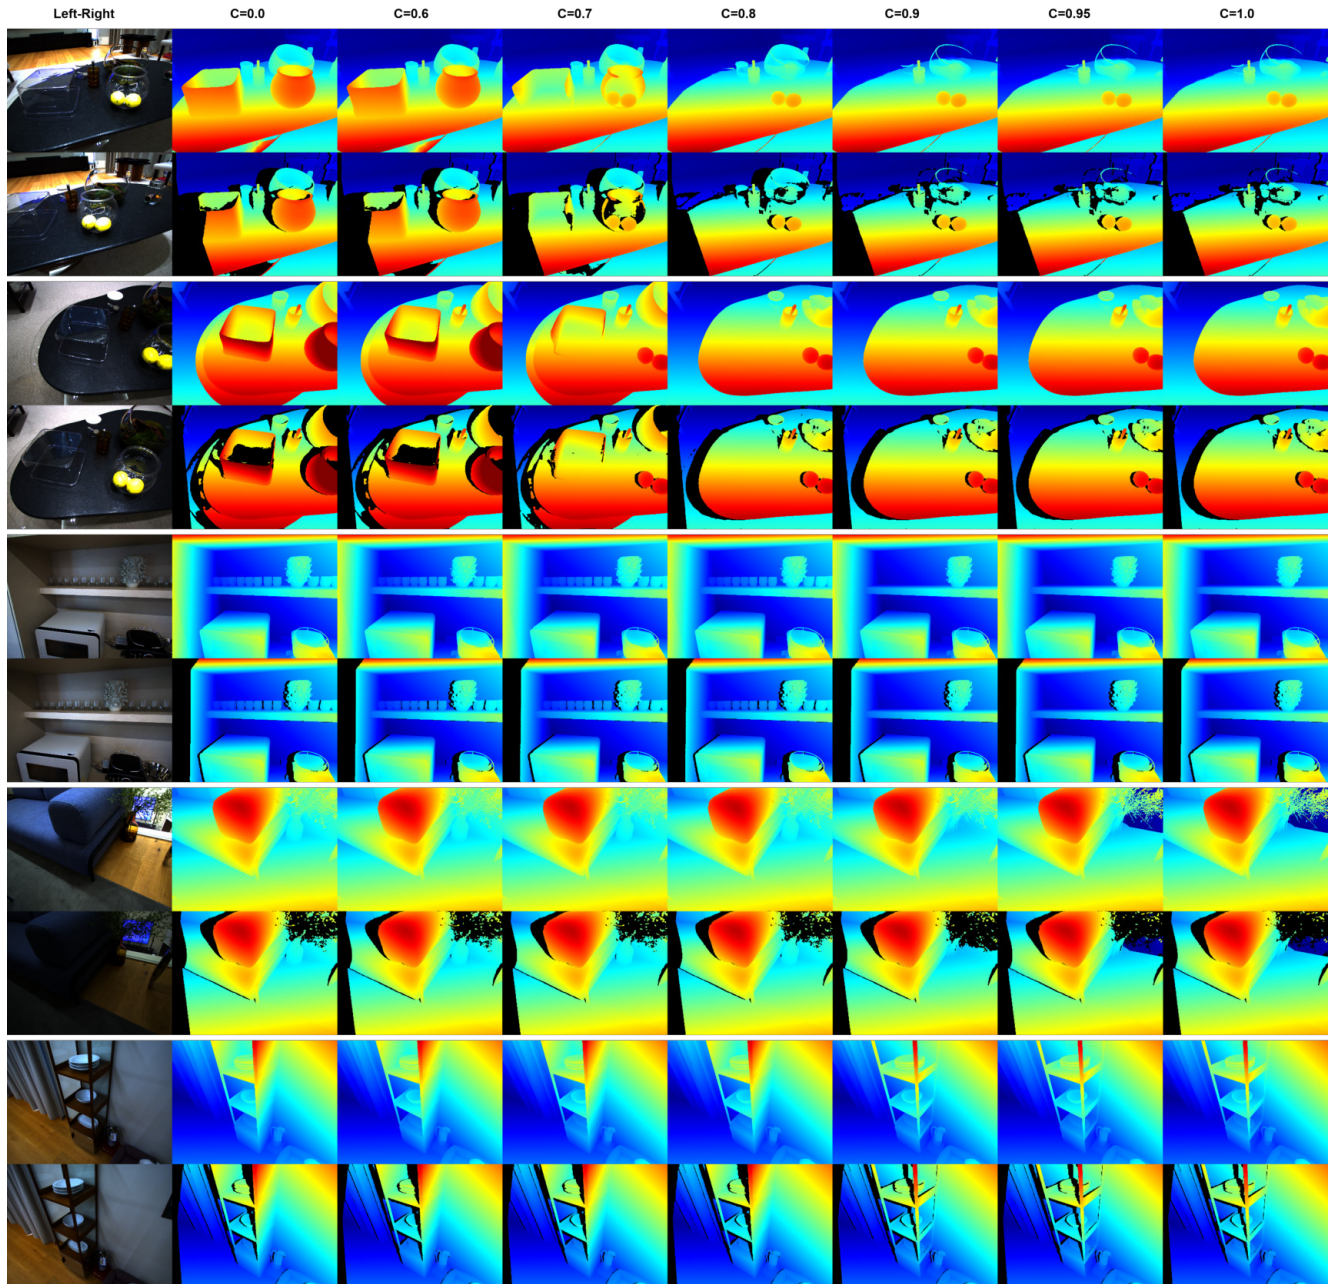

Figure 12. **Generalization to real-world scenes (2).** Results on scenes containing multiple transparent objects, including transparent plastic bowls and glass cups. Our model effectively resolves the depth ambiguity inherent in these materials, allowing for selective reconstruction of the transparent surfaces or the background behind them according to the user intent parameter  $c$ .

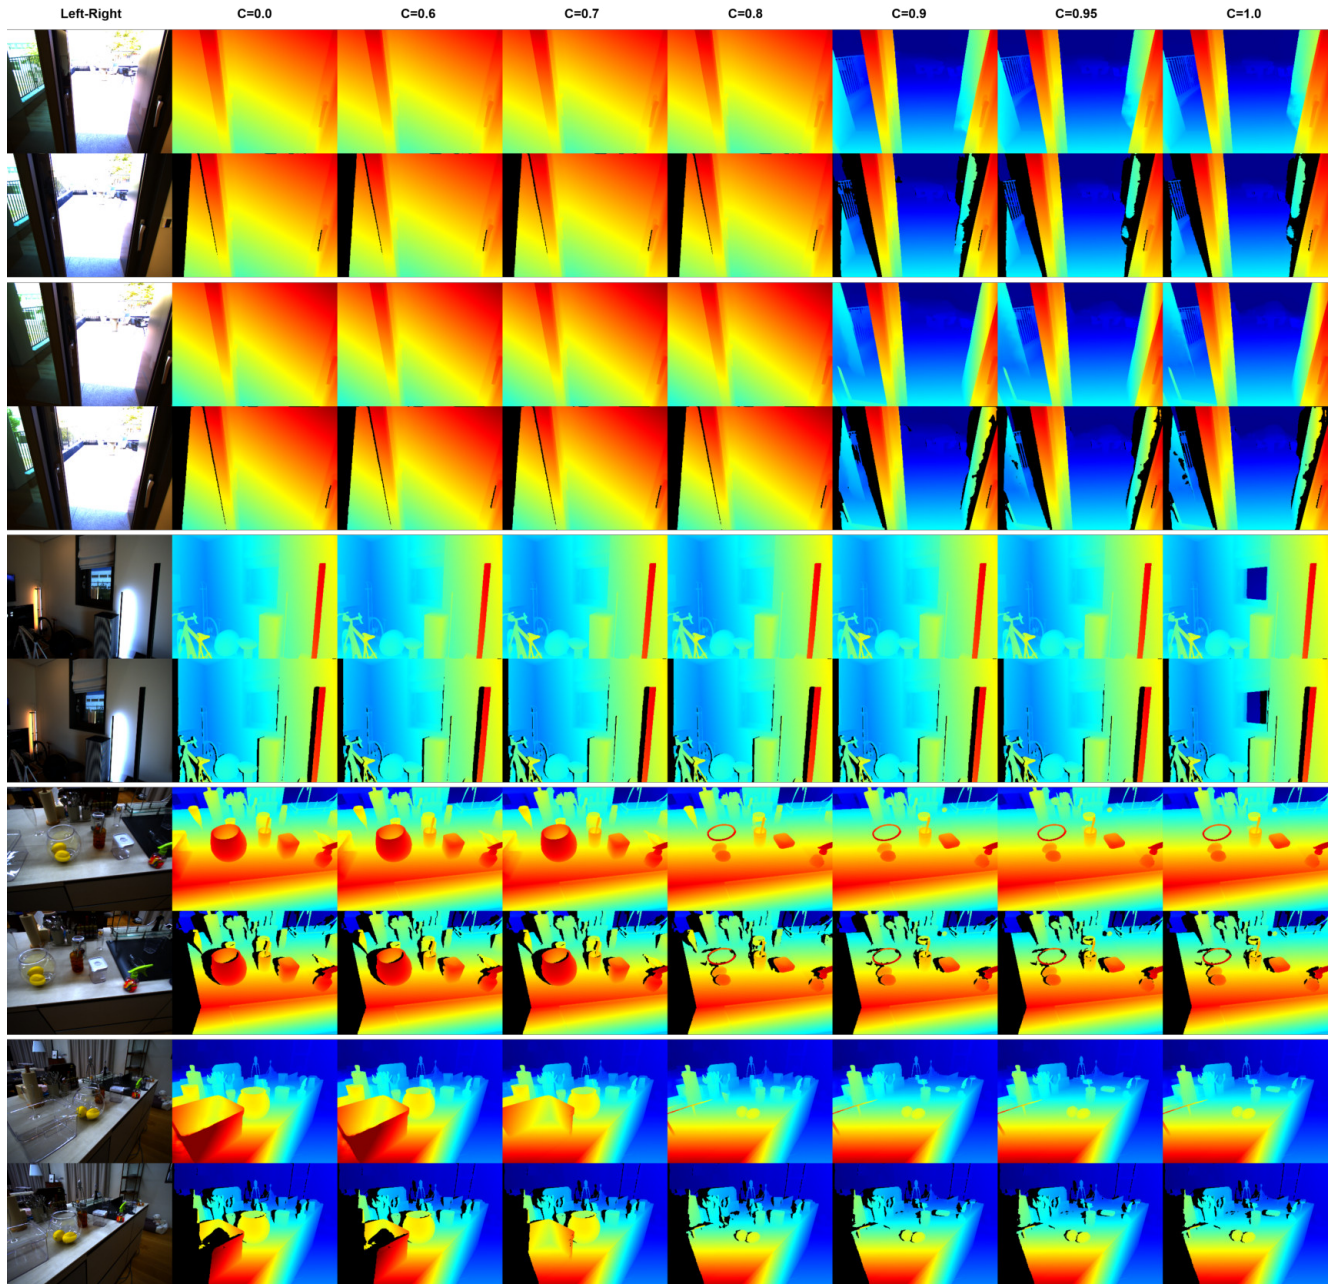

Figure 13. **Generalization to real-world scenes (3).** Results on challenging scenes containing thin structures and complex lighting. The model successfully recovers the depth of a window insect screen (mosquito net). Furthermore, it maintains robustness in high-contrast scenarios, such as indoor views looking outdoors where regions exhibit strong saturation.

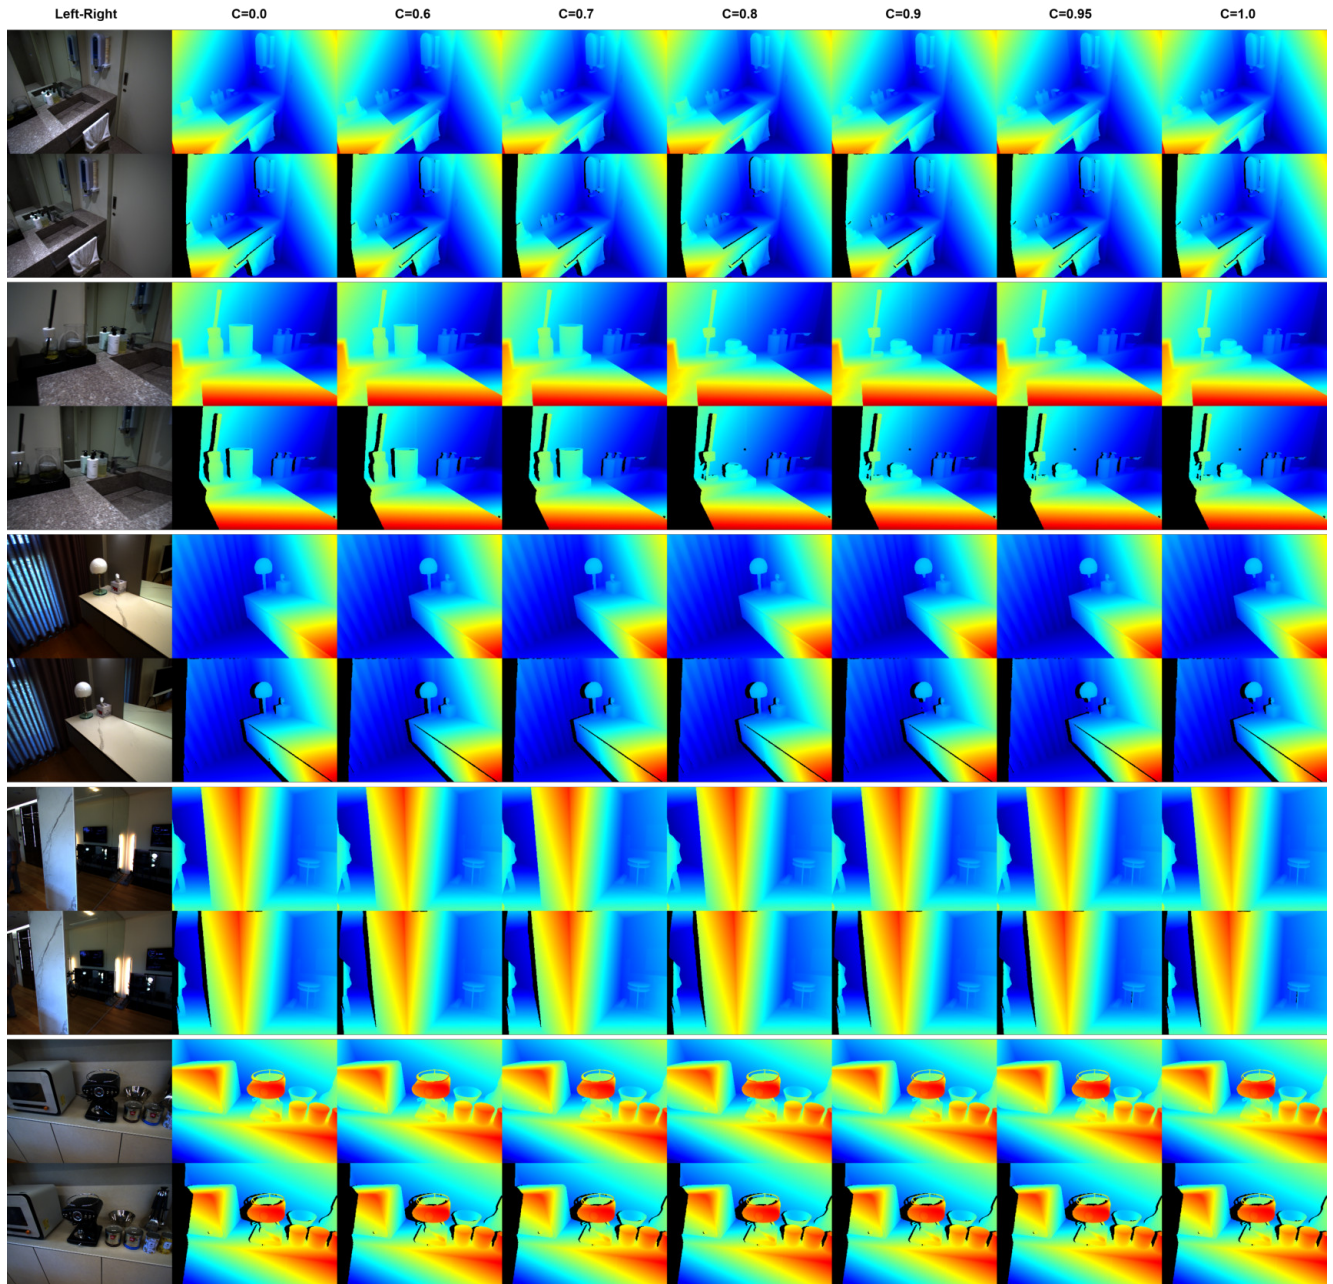

Figure 14. **Robustness on mirrors and highly reflective surfaces.** Unlike transparent scenes where depth varies with user intent, our model exhibits robustness on mirrors (e.g., bathroom and wall mirrors). It consistently estimates the physical surface distance regardless of the parameter  $c$ , correctly avoiding the estimation of virtual depth from reflected objects.

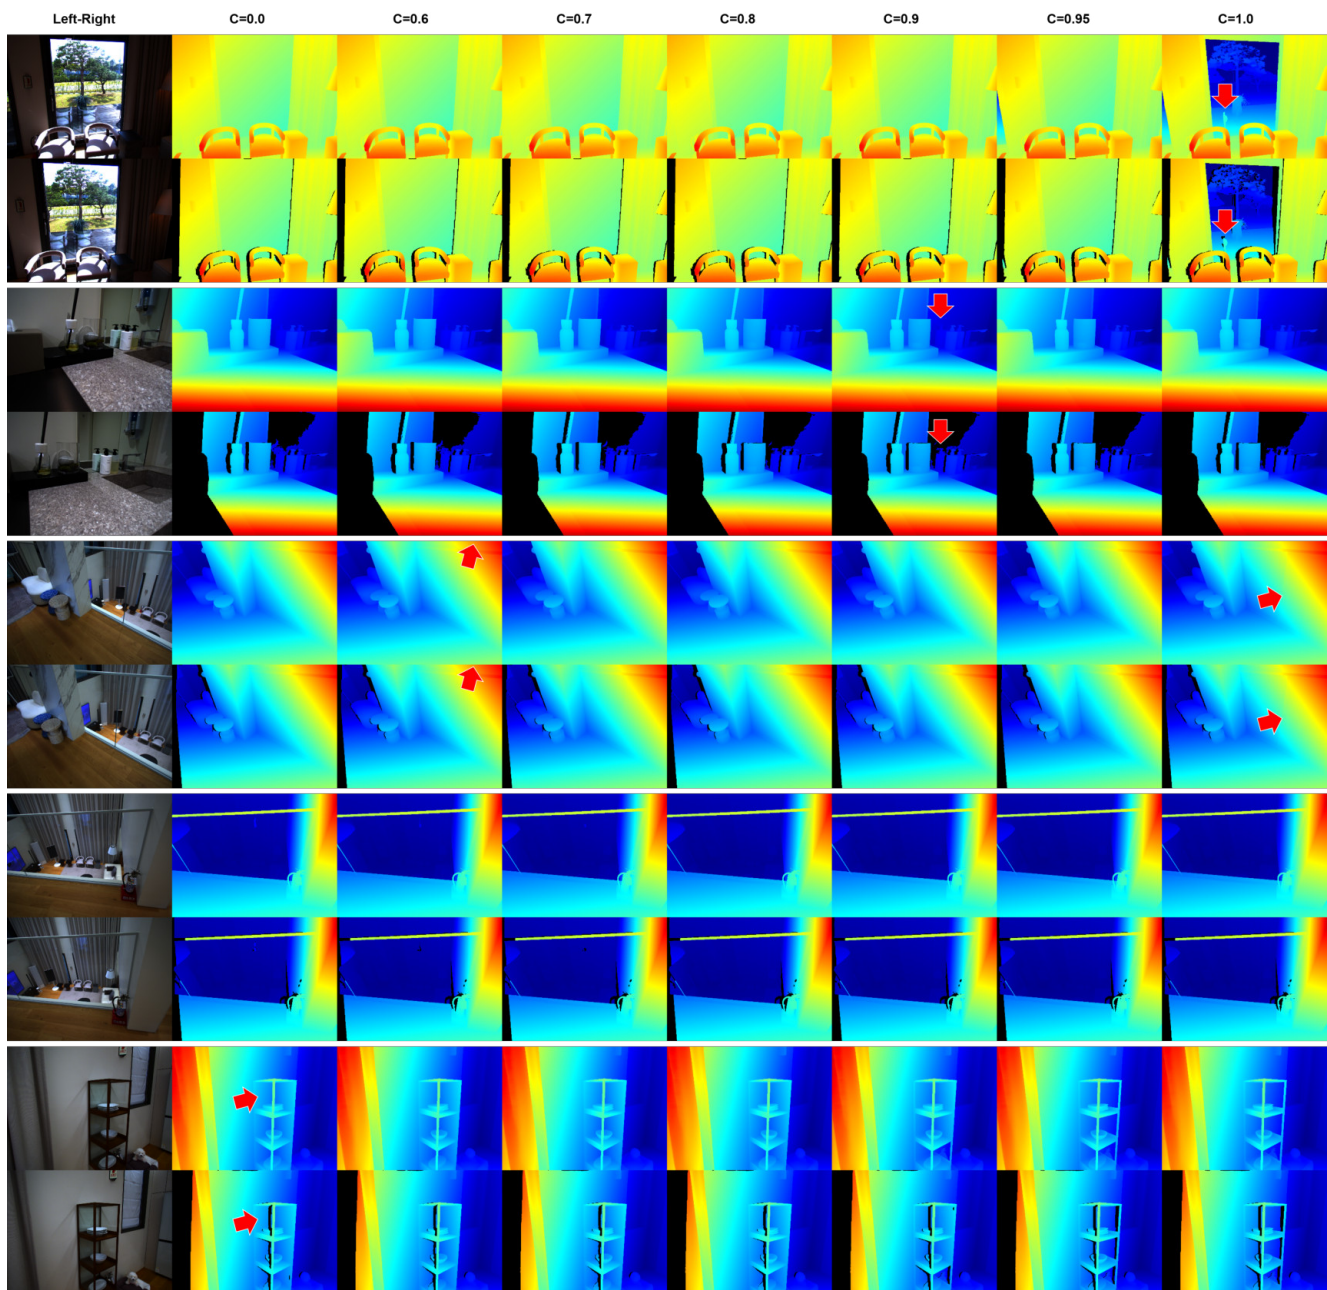

Figure 15. **Failure cases analysis.** We present typical limitation scenarios: (1) Missed detections on highly transparent objects such as glass fences or clear windows. (2) View-dependent inconsistencies: even objects successfully detected in other views (e.g., furniture glass) may be missed from specific angles. (3) Floating artifacts appearing in mid-air (e.g., on window glass) when reflection and transmission intensities are comparable. (4) Occasional estimation of virtual depth (i.e., distance to the reflected object) in mirrors.

## References

- [1] Blenderkit. <https://www.blenderkit.com/>.
- [2] Adrien Gaidon, Qiao Wang, Yohann Cabon, and Eleonora Vig. Virtual worlds as proxy for multi-object tracking analysis. In *Proceedings of the IEEE/CVF Conference on Computer Vision and Pattern Recognition*, pages 4340–4349, 2016.
- [3] Mark Edward M. Gonzales, Lorene C. Uy, and Joel P. Ilao. Designing a lightweight edge-guided convolutional neural network for segmenting mirrors and reflective surfaces. *Computer Science Research Notes*, 3301:107–116, 2023.
- [4] Jiankun Li, Peisen Wang, Pengfei Xiong, Tao Cai, Ziwei Yan, Lei Yang, Jiangyu Liu, Haoqiang Fan, and Shuaicheng Liu. Practical stereo matching via cascaded recurrent network with adaptive correlation. In *Proceedings of the IEEE/CVF Conference on Computer Vision and Pattern Recognition*, pages 16263–16272, 2022.
- [5] Jiaying Lin, Yuen Hei Yeung, and Rynson WH Lau. Exploiting semantic relations for glass surface detection. In *Proc. NeurIPS*, 2022.
- [6] Jiaying Lin, Xin Tan, and Rynson WH Lau. Learning to detect mirrors from videos via dual correspondences. In *Proceedings of the IEEE/CVF conference on computer vision and pattern recognition*, pages 9109–9118, 2023.
- [7] Nikolaus Mayer, Eddy Ilg, Philip Hausser, Philipp Fischer, Daniel Cremers, Alexey Dosovitskiy, and Thomas Brox. A large dataset to train convolutional networks for disparity, optical flow, and scene flow estimation. In *Proceedings of the IEEE/CVF Conference on Computer Vision and Pattern Recognition*, pages 4040–4048, 2016.
- [8] Junhong Min and Youngpil Jeon. Confidence aware stereo matching for realistic cluttered scenario. In *2024 IEEE International Conference on Image Processing (ICIP)*, pages 3491–3497. IEEE, 2024.
- [9] Junhong Min, Youngpil Jeon, Jimin Kim, and Minyong Choi. S<sup>2</sup>M<sup>2</sup>: Scalable stereo matching model for reliable depth estimation. *arXiv preprint arXiv:2507.13229*, 2025.
- [10] Pierluigi Zama Ramirez, Fabio Tosi, Matteo Poggi, Samuele Salti, Stefano Mattoccia, and Luigi Di Stefano. Open challenges in deep stereo: the booster dataset. In *Proceedings of the IEEE/CVF Conference on Computer Vision and Pattern Recognition*, pages 21168–21178, 2022.
- [11] Daniel Scharstein, Heiko Hirschmüller, York Kitajima, Greg Krathwohl, Nera Nešić, Xi Wang, and Porter Westling. High-resolution stereo datasets with subpixel-accurate ground truth. In *Pattern Recognition: 36th German Conference, GCPR 2014, Münster, Germany, September 2-5, 2014, Proceedings 36*, pages 31–42. Springer, 2014.
- [12] Thomas Schops, Johannes L Schonberger, Silvano Galliani, Torsten Sattler, Konrad Schindler, Marc Pollefeys, and Andreas Geiger. A multi-view stereo benchmark with high-resolution images and multi-camera videos. In *Proceedings of the IEEE/CVF Conference on Computer Vision and Pattern Recognition*, pages 3260–3269, 2017.
- [13] Fabio Tosi, Yiyi Liao, Carolin Schmitt, and Andreas Geiger. Smd-nets: Stereo mixture density networks. In *Proceedings of the IEEE/CVF Conference on Computer Vision and Pattern Recognition*, pages 8942–8952, 2021.
- [14] Jonathan Tremblay, Thang To, and Stan Birchfield. Falling things: A synthetic dataset for 3d object detection and pose estimation. In *Proceedings of the IEEE/CVF Conference on Computer Vision and Pattern Recognition Workshops*, pages 2038–2041, 2018.
- [15] Qiang Wang, Shizhen Zheng, Qingsong Yan, Fei Deng, Kaiyong Zhao, and Xiaowen Chu. Irs: A large naturalistic indoor robotics stereo dataset to train deep models for disparity and surface normal estimation. In *IEEE International Conference on Multimedia and Expo (ICME)*, pages 1–6. IEEE, 2021.
- [16] Wenshan Wang, DeLong Zhu, Xiangwei Wang, Yaoyu Hu, Yuheng Qiu, Chen Wang, Yafei Hu, Ashish Kapoor, and Sebastian Scherer. Tartanair: A dataset to push the limits of visual slam. In *IEEE/RSJ International Conference on Intelligent Robots and Systems (IROS)*, pages 4909–4916. IEEE, 2020.
- [17] Bowen Wen, Matthew Trepte, Joseph Aribido, Jan Kautz, Orazio Gallo, and Stan Birchfield. Foundationstereo: Zero-shot stereo matching. In *Proceedings of the Computer Vision and Pattern Recognition Conference*, pages 5249–5260, 2025.
- [18] Mingchen Xu, Peter Herbert, Yu-Kun Lai, Ze Ji, and Jing Wu. Rgb-d video mirror detection. In *2025 IEEE/CVF Winter Conference on Applications of Computer Vision (WACV)*, pages 9640–9649. IEEE, 2025.
- [19] Guorun Yang, Xiao Song, Chaoqin Huang, Zhidong Deng, Jianping Shi, and Bolei Zhou. Drivingstereo: A large-scale dataset for stereo matching in autonomous driving scenarios. In *Proceedings of the IEEE/CVF Conference on Computer Vision and Pattern Recognition*, pages 899–908, 2019.
